# Supplementary material for: Weight-Space Programming for Medical Imaging: Do We Still Need Training Data?
Source: arXiv:2611.12066 source file (2026-11-09)
Supplement: Supplementary file 1 [file supplementary.tex]

% CVPR supplementary material (anonymous). The arXiv version appends the same file to main.pdf.
\documentclass[10pt,twocolumn,letterpaper]{article}
\usepackage[review]{cvpr}
\input{preamble}
\renewcommand{\ttdefault}{lmtt}
\makeatletter\newcommand{\tabinput}[1]{\@@input #1 }\makeatother
\input{tables/numbers}
\definecolor{cvprblue}{rgb}{0.21,0.49,0.74}
\usepackage[pagebackref,breaklinks,colorlinks,allcolors=cvprblue]{hyperref}
\def\paperID{*****}\def\confName{CVPR}\def\confYear{2027}
\title{Weight-Space Programming for Medical Imaging:\\Do We Still Need Training Data?\\[4pt]
\large Supplementary Material}
\author{Anonymous CVPR submission\\Paper ID \paperID}
\begin{document}
\maketitle
\input{sec/6_supp}
{\small\bibliographystyle{ieeenat_fullname}\bibliography{main}}
\end{document}
